# Supplementary material for: Improving Language Models via Plug-and-Play Retrieval Feedback
Source: arXiv:2305.14002 source file (2023-05-23)
Supplement: Supplementary file 1 [file 6-appendix.tex]

\begin{table*}[h]
\centering
\setlength{\tabcolsep}{2mm}{
\begin{tabular}{l|lrrrc}
\toprule
Datasets & Splits & Train & Valid & Test & Test labels \\
\midrule
\multirow{2}{*}{TriviaQA~\citep{joshi2017triviaqa}} & open domain & 78,785 & 8,837 & 11,313 & public  \\
& wikipedia split &  &  & 7,993 & public  \\
WebQ~\citep{berant2013semantic} & open domain & 3,478 & 300 & 2,032 & public \\
NQ~\citep{kwiatkowski2019natural} & open domain & 79,168 & 8,757 & 3,610 & public \\
FEVER~\citep{thorne2018fever} & kilt challenge & 104,966 & 10,444 & 10,100 & hidden \\
FM2~\citep{eisenschlos2021fool} & official split & 10,149 & 1169 & 1380 & public \\
WoW~\citep{dinan2019wizard} & kilt challenge & 63,734 & 3,054 & 2,944 & hidden \\
\bottomrule
\end{tabular}}
\vspace{-0.08in}
\caption{Datasets splits and statistics. For FEVER and WoW, labels in the test are hidden, so the model performance should be evaluated at \url{https://ai.facebook.com/tools/kilt/}.}
\label{tab:coverage}
\end{table*}

\subsection{Datasets and Splits}
\label{sec:datasets}

-- \textsc{TriviaQA} (TQA)~\citep{joshi2017triviaqa} contains a set of trivia questions with answers that were originally scraped from trivia and quiz-league websites.

-- \textsc{WebQuestions} (WebQ)~\citep{berant2013semantic} consists of questions selected using Google Suggest API,
where the answers are entities in Freebase.

-- \textsc{Natural Questions} (NQ)~\citep{kwiatkowski2019natural} were mined from real Google search queries and the answers are spans in Wikipedia articles identified by human annotators. 

We explore the same train / dev / test splits for the open-domain QA setting as used by \cite{izacard2021leveraging,karpukhin2020dense}. 
For TriviaQA, GPT-3 / GLaM / PaLM~\citep{brown2020language,du2022glam,chowdhery2022palm} evaluate on the Wikipedia dev set of 7,993 examples, so we ran an additional evaluation on that dev set in order to compare with their performance.

-- \textsc{Fever}~\citep{thorne2018fever} is one of the largest datasets for fact checking that requires retrieving  evidence from external corpus to support if a statement is supported or refuted.

-- \textsc{Fool Me Twice} (FM2)~\citep{eisenschlos2021fool} is a challenging fact checking dataset collected by gamification. Players write challenging claims either entailed or refuted by evidence from Wikipedia. They are then tasked to spot the refuted claim among a group.

-- \textsc{Wizard of Wikipedia} (WoW)~\citep{dinan2019wizard} is an open-domain dialogue task for training agents that can converse knowledgeably about open-domain topics. 
One speaker in the conversation must ground their utterances in a specific knowledge sentence from a Wikipedia page. 

We use the same train / dev / test splits in KILT challenge~\citep{petroni2021kilt} for the FEVER and WoW datasets. Their test labels are hidden, so the performance can only be evaluated through \url{https://ai.facebook.com/tools/kilt}. For FM2, we use its official dataset splits.
